# Supplementary material for: Delving into Masked Autoencoders for Multi-Label Thorax Disease Classification
Source: arXiv:2210.12843 source file (2022-10-23)
Supplement: Supplementary file 1 [file 8_appendix.tex]

\clearpage
\appendix

\begin{table*}[b]
\centering
    \footnotesize
    \begin{tabular}{p{0.13\linewidth}|P{0.05\linewidth}P{0.05\linewidth}P{0.05\linewidth}|P{0.13\linewidth}P{0.13\linewidth}|P{0.13\linewidth}P{0.13\linewidth}}
        \hline
         & \multicolumn{3}{c|}{Size (\# of px)} & \multicolumn{2}{c|}{DenseNet-121} & \multicolumn{2}{c}{ViT-S/16} \\
        \
        Disease & Mean & Q1 & Q3 & AP$_{25}$ (95\% CI) & AP$_{50}$ (95\% CI) & AP$_{25}$ (95\% CI) & AP$_{50}$ (95\% CI) \\
        \shline
        Atelectasis & 924 & 567 & 2016 & 10.1 {\footnotesize (9.8--10.1)} & 2.0 {\footnotesize (1.9--2.0)} & 31.5 {\footnotesize (31.5--31.9)} & 8.1 {\footnotesize (7.9--8.1)} \\
        Cardiomegaly & 8670 & 7563 & 10050 & 89.6 {\footnotesize (89.4--89.7)} & 53.3 {\footnotesize (53.3--53.7)} & 16.3 {\footnotesize (16.2--16.4)} & 3.0 {\footnotesize (2.9--3.0)} \\ 
        Effusion & 2925 & 1426 & 5042 & 24.5 {\footnotesize (24.3--24.7)} & 2.9 {\footnotesize (2.9--3.1)} & 8.8 {\footnotesize (8.6--8.9)} & 1.0 {\footnotesize (0.9--1.0)} \\
        Infiltrate & 2754 & 1746 & 4878 & 32.9 {\footnotesize (32.6--33.1)} & 12.7 {\footnotesize (12.6--12.9)} & 11.4 {\footnotesize (11.3--11.6)} & 1.3 {\footnotesize (1.3--1.3)} \\
        Mass & 756 & 494 & 1980 & 25.4 {\footnotesize (25.2--25.7)} & 1.6 {\footnotesize (1.4--1.6)} & 27.0 {\footnotesize (26.8--27.5)} & 11.1 {\footnotesize (10.9--11.3)} \\
        Nodule & 224 & 152 & 332 & 0.0 {\footnotesize (0.0--0.0)} & 0.0 {\footnotesize (0.0--0.0)} & 9.2 {\footnotesize (9.1--9.4)} & 3.9 {\footnotesize (3.9--4.1)} \\
        Pneumonia & 2944 & 1850 & 4628 & 32.0 {\footnotesize (31.7--32.1)} & 6.2 {\footnotesize (6.0--6.2)} & 27.8 {\footnotesize (27.6--28.1)} & 9.3 {\footnotesize (9.1--9.4)} \\
        Pneumothorax & 1899 & 917 & 4064 & 11.6 {\footnotesize (11.5--11.8)} & 2.3 {\footnotesize (2.3--2.4)} & 4.7 {\footnotesize (4.5--4.7)} & 0.0 {\footnotesize (0.0--0.0)} \\
        \hline
        All eight diseases & 2300 & 755 & 5985 & 31.0 {\footnotesize (30.9--31.1)} & 12.3 {\footnotesize (12.3--12.4)} & 18.0 {\footnotesize (18.0--18.1)} & 4.7 {\footnotesize (4.7--4.7)} \\
        \hline
    \end{tabular}

    \caption{
        \textbf{Weakly-supervised localization of eight diseases.} 
        We report average precision (AP) on 25\% and 50\% IoUs, associated with 95\% confidence intervals for 100 different trials. The IoU is calculated between the ground truth bonding box and bounding box of the largest connected component in the Grad-CAM heatmap.
        We also present the statistics (mean, 25th and 75th percentiles) of ground truth bounding box sizes of each disease, measured by the number of pixels within the bounding box.
        Combining disease size statistics and AP performance, we observe that CNN can detect large diseases (\eg Cardiomegaly, Pneumonia) significantly better than ViT, while ViT can capture small diseases (\eg nodule).
        The statistical analysis shows that the performance difference between DenseNet-121 and Vit-S/16 is significant.
        Qualitative visualization is presented in~\figureautorefname~\ref{fig:appendix_grad_cam}.
    }
    \label{tab:appendix_detection_results}
\end{table*}

\noindent\textbf{Abstract.} This document provides the supplementary material for the paper entitled ``Delving into Masked Autoencoders for Multi-Label Chest X-ray Classification''.
The supplementary material mainly investigates the explainability of CNN and ViT, organized as follows:
\S\ref{sec:appendix_gradcam_details} describes the implementation details of weakly-supervised disease localization performed by CNN and ViT;
\S\ref{sec:appendix_detection_results} presents the results of CNN and ViT in weakly-supervised localization of eight diseases;
and \S\ref{sec:appendix_gradcam_visualizations} contains a qualitative visualization on disease localization using Grad-CAM~\cite{selvaraju2017grad} heatmaps.

\section{Implementation Details}
\label{sec:appendix_gradcam_details}
The \textit{grad-cam} package\footnote{\href{https://github.com/jacobgil/pytorch-grad-cam}{github.com/jacobgil/pytorch-grad-cam}}~\cite{jacobgilpytorchcam} was used to generate Grad-CAM heatmaps~\cite{selvaraju2017grad} for both CNN and ViT.  We use the last dense-block (4th) of DenseNet-121 and the LayerNorm layer in the last transfomer block (12th) of ViT-S/16  as the ``target layers'' for Grad-CAM. We use default settings for other hyper-parameters. The experiments are done with a small subset of the NIH ChestX-ray14 dataset, which includes 787 cases with official bounding-box annotations of a total of eight chest diseases. The final predicted bounding-box of the diseased region is generated with the thresholded Grad-CAM heatmap, largest connected component, and box regression.

\section{Weakly-supervised Localization Results}
\label{sec:appendix_detection_results}

Based on the IOUs of each pair of Grad-CAM generated bound box and the ground truth bounding box, we use Average Precision (AP) as the detection metric~\cite{lin2014microsoft}. Precision is defined as $tp/(tp+fp)$, where $tp$ and $fp$ denote the number of true positives and false positives, respectively.
AP$_{25}$ considers cases with IoU$>$25\% as true positives and $AP_{50}$ with IoU$>$50\%. \Cref{tab:appendix_detection_results} shows the detection results (including disease-wise results and all diseases) of DenseNet-121 and ViT-S/16. 
In addition, we present the statistics of bounding box size (measured by the number of pixels in the box) for each disease.
We can clearly see that the CNN provides better localization explainability on diseases in large size (\eg Cardiomegaly and Pneumonia) while ViT is robust to diseases in small size (\eg Nodule). Regarding the general results of all diseases, CNN significantly exceeds the localization ability (31.0\%~vs.~18.0\%, AP$_{25}$; 12.3\%~vs.~4.7\%, AP$_{50}$) to ViT with the Grad-CAM heatmap. This study suggests that class activation maps are more suitable for visualizing the explainability of CNN-type models. In the future, other than class activation maps, we will seek to explore the explainability for Vision Transformers in multi-label classification tasks, with the help of self-attention derived from the Transformer architectures~\cite{caron2021emerging,raghu2021vision,abnar2020quantifying,chefer2021transformer}.

\section{Class Activation Maps Visualization}
\label{sec:appendix_gradcam_visualizations}

\Cref{fig:appendix_grad_cam} provides examples of class activation maps predicted by DenseNet-121 and ViT-S/16. With the help of Grad-CAM, we are able to check which part of the X-ray image is responsible for the model prediction (the diseased region).
To ensure an objective comparison, we display the visualizations into three groups---best in CNN, best in ViT, and both poor in CNN and ViT---from left to right in \Cref{fig:appendix_grad_cam}. The results are evaluated by IoU between ground truth bounding box and the bounding box of the largest connected component in the attention response. Based on our results, CNN outperforms ViT on the diseases that have a large infected region (\eg Cardiomegaly) while ViT shows better robustness to disease that occur in small regions (\eg Nodule).

\begin{figure*}[htbp]
    \centering
    \includegraphics[width=1.0\linewidth]{Figures/fig_grad_cam.pdf}
    \caption{\textbf{Grad-CAM visualization of CNN and ViT.} NIH ChestX-ray14 provides disease bounding boxes of 787 chest X-rays, as shown in white boxes.
    Left, middle, and right panels display successful cases predicted by CNN, ViT, and both failure cases for each disease, respectively.
    Although the classification performance of CNN and ViT is comparable (82.1\%~vs.~82.3\% AUC), their attention maps generated by Grad-CAM behave differently.
    Attentions in CNN are relatively larger and more concentrated than those in ViT.
    This observation is consistent with those in Chefer~\etal~\cite{chefer2021transformer}.
    In general, CNN and ViT perform fairly well in weakly-supervised localizing diseases that have large infected regions (\eg Cardiomegaly, Pneumonia, Pneumothorax), but fail in small abnormalities (\eg tiny Nodule and Effusion). [Better viewed on-line, in color, and zoomed in for details]
    }
    \label{fig:appendix_grad_cam}
\end{figure*}
